# Supplementary material for: Know your sensORs -- A Modality Study For Surgical Action Classification
Source: arXiv:2203.08674 source file (2022-09-18)
Supplement: Supplementary file 1 [file 07_suppl.tex]

\section{Supplementary Material}

\begin{figure}[H]
  \centering
    \includegraphics[width=0.99\textwidth]{"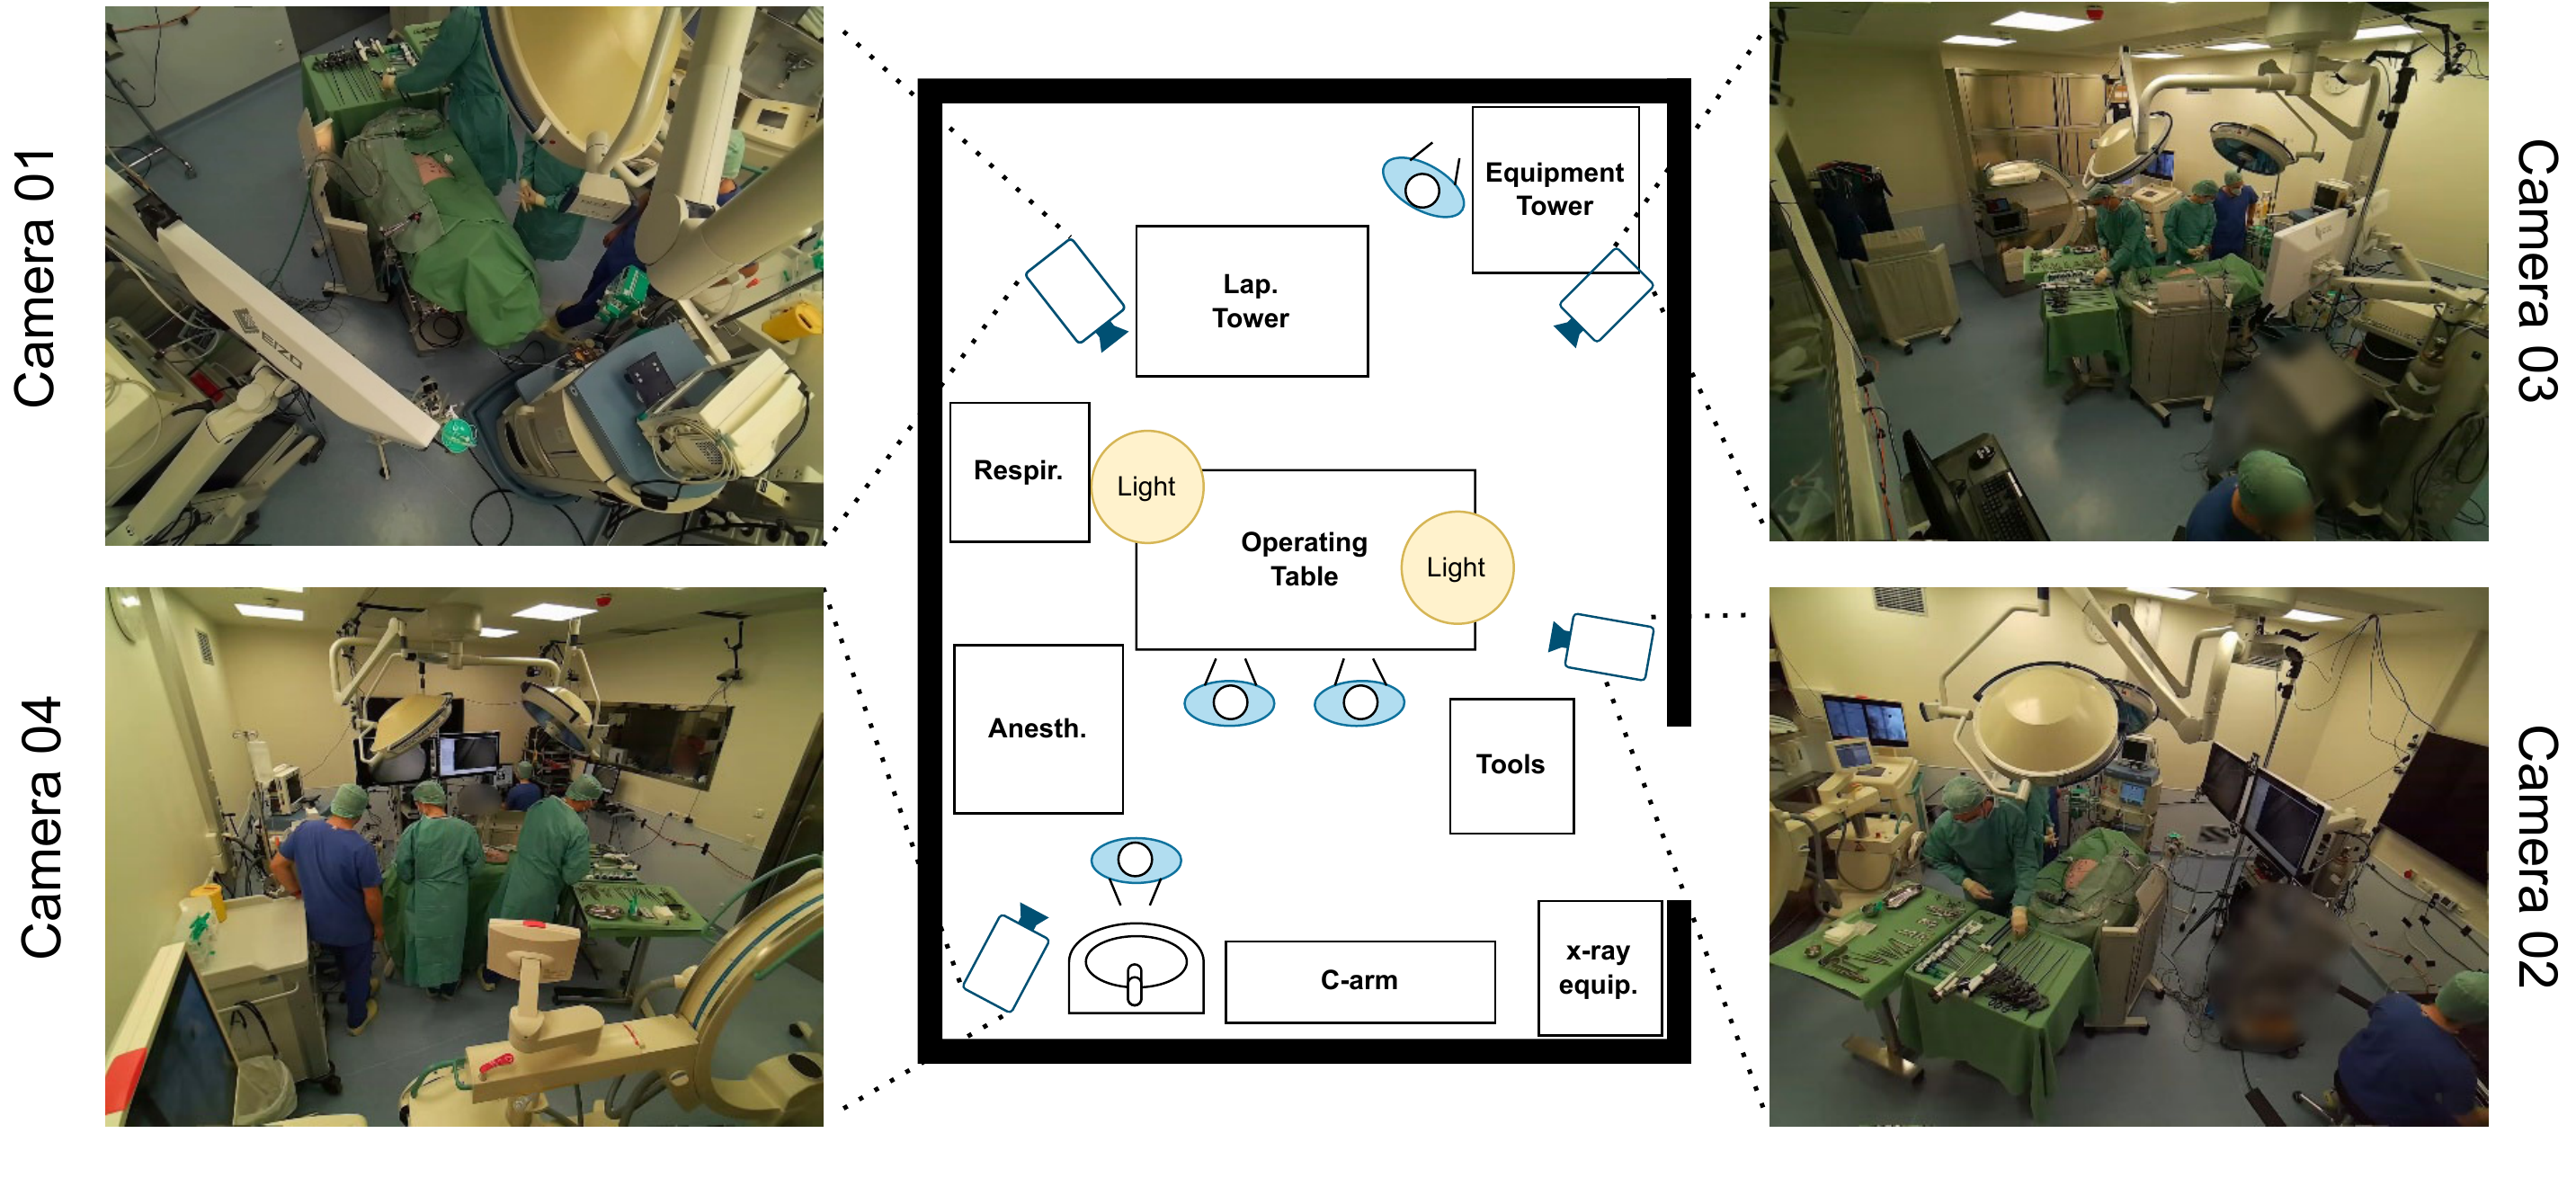"}%
  \caption{\textbf{Multi-view OR Dataset}. Complete multi-view OR acquisitions with 4 cameras. We evaluate two additional workflow views (cameras 03 and 04).}
  \label{fig:or_cameras}
\end{figure}

\begin{table}[H]
\setlength{\tabcolsep}{7pt}

\centering
\caption{Comparison of two additional workflow cameras (see Fig. \ref{fig:or_cameras}). The trends observed are consistent with those of cameras 01 and 02.}
\label{tab1}
\begin{tabular}{l  c  c  c  c | c c c c}
\toprule
  & \multicolumn{4}{c|}{Camera 03 (Workflow)} & \multicolumn{4}{c}{Camera 04 (Workflow)} \\
  & \multicolumn{2}{c}{ResNet} & \multicolumn{2}{c|}{X3D\_M} & \multicolumn{2}{c}{ResNet} & \multicolumn{2}{c}{X3D\_M} \\
\midrule
  Modality & acc. & mAP & acc. & mAP & acc. & mAP & acc. & mAP\\
\midrule
  RGB        & 88.1 & 96.0 & 89.9 & 97.3 % camera 03 == 03
             & 75.9 & 81.3 & 79.1 & 86.8 \\ % camera 04 == 01
  Depth      & 65.4 & 74.0 & 85.5 & 93.7
             & 60.7 & 64.5 & 75.2 & 85.3 \\
  IR         & 76.0 & 68.6 & 78.3 & 87.8
             & 53.5 & 55.0 & 69.2 & 69.1 \\
\midrule
  IR+Depth${}^{\text{ef}}$   & 69.3 & 77.3 & 78.0 & 84.5
             & 58.6 & 60.5 & 73.9 & 83.4 \\             
  RGB+Depth${}^{\text{ef}}$
             & 88.0 & 92.5 & 90.0 & 97.1
             & 69.2 & 73.8 & 78.9 & 89.6 \\
%\midrule
  RGB+Depth${}^{\text{lf}}$
             & 85.8 & 95.1 & \textbf{94.4} & \textbf{98.9}
             & 76.1 & 85.8 & \textbf{83.6} & \textbf{93.09} \\
\bottomrule
\end{tabular}
\end{table}

\begin{figure}
    \centering
    \includegraphics[width=0.6\textwidth]{"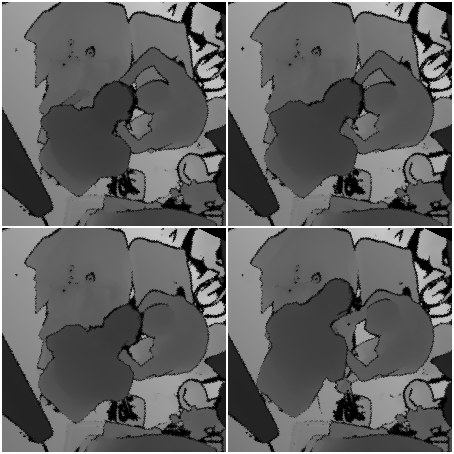"}
    \caption{\textbf{Sample depth image sequence.} We use 16-frame clips spanning four seconds as inputs for the X3D architecture. The model was adapted to handle varying input modalities.}
    \label{fig:my_label}
\end{figure}

\begin{figure}
  \centering
    \includegraphics[width=0.6\textwidth]{"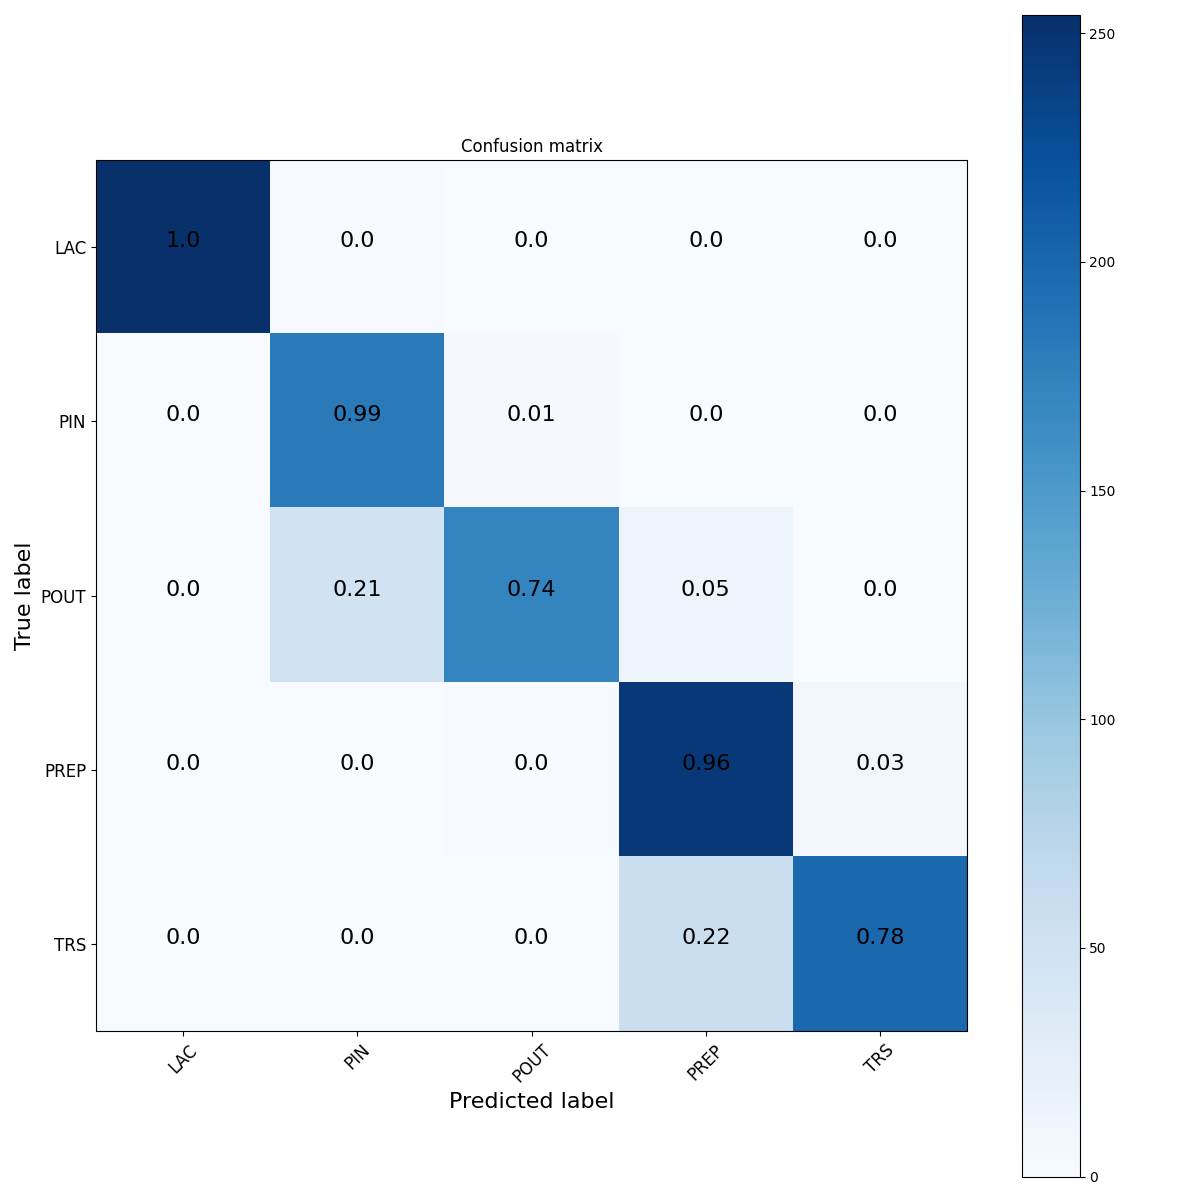"}%
  \caption{\textbf{Sample Confusion Matrix}. Camera 02 (Workflow), late fusion of RGB and depth with the X3D\_M architecture. "PIN" and "POUT" as well as "PREP" and "TRS" are not distinguished as well as "LAC".}
  \label{fig:confusion_matrix}
\end{figure}
